# Supplementary material for: Performative Recommendation: Diversifying Content via Strategic Incentives
Source: arXiv:2302.04336 source file (2023-06-08)
Supplement: Supplementary file 1 [file appendix.tex]

\section{Optimization}
\subsection{Best response} \label{apx:best_response}
\proof
To compute an item's best-response update,
it suffices to solve the following constrained problem:\\
\begin{align*}
& \max_{x'} v^Tx' - \alpha c(x', x) \quad \textrm{s.t} \quad ||x||_2=1 &   \\
% & \max_{x'} v^Tx' - \alpha \|x' - x\|_2^2 \quad \textrm{s.t} \quad ||x||_2=1 &   \\
\intertext{where $c(x,x')=\|x'-x\|_2^2$.
We solve for $x'$ using Lagrangian analysis.
First, we square the constraint (which does not change the condition itself). 
Define the Lagrangian as follows:}
&L(x', \lambda) =  v^Tx' - \alpha\|x' - x\|_2^2 +\lambda[||x'||_2^2-1] &
\intertext{Next, to find the minimum of $L$, derive with respect to $x'$, and compare to 0:}
& v - 2\alpha(x' - x) + 2\lambda x' = 0  \\
& v + 2\alpha x = 2\alpha x' - 2\lambda x' \\
& \frac{v + 2\alpha x}{2\alpha - 2\lambda} = x' &
\intertext{Plugging $x'$ into the original constraint gives:}
& \frac{|v+2\alpha x|}{|2\alpha - 2\lambda|} = 1 \\
& |v+2\alpha x| = 2\alpha -2\lambda \\
& |v+2\alpha x| - 2\alpha = -2\lambda & \\
\intertext{Finally, plugging $\lambda$ into the expression for $x'_i$ obtains:}
& \frac{v +2\alpha x}{|v+2\alpha x|} = x'
\end{align*}

\section{Proofs}
\subsection{proposition 1}
\label{apx:proof_full_users_overlap}
\proof
As both items have the same set of users, the normalized average of users embedded is the same for both items. We denote normalized average of users embedded by $\vtilde$. Since there is no limitation for the modification $\alpha=0$ the best response (according to equation \eqref{eq:Delta_closed_form}) is to change the item vector feature to $\vtilde$. 
As a result both item will be changed to the same point which means dissimilarity of 0 between them.
\endproof
\subsection{empirical generalization of proposition 1 to $\alpha \ne 0$ cases}
\label{apx:empirical_generalization_full_overlapping}
\begin{figure}[t!]
\centering
        \includegraphics[width=0.5\linewidth]{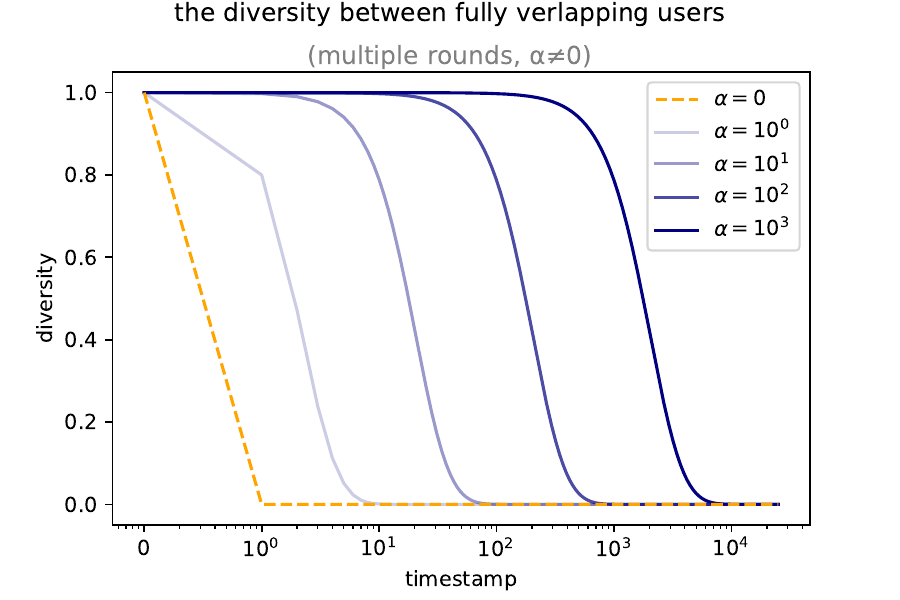}
 \caption{Empirical evidence for proposition 1 when $\alpha \ne 0$}
\label{fig:prop_full_overlapping_diff_a}
\end{figure}

Here we proposed empirical evidence that proposition 1 holds for $\alpha \ne 0$. However, it may take many rounds for the diversity to drop to 0. In order to test our claim we ran synthetic 2 dimensional experiment. We placed two items so that they were as far apart as possible, i.e. one at (1,0) and the other at (-1, 0). We randomly choose direction that represents $\vtilde$ the spherical average of the overlap users. We measure how the diversity change over the time. The experiment results are shown in figure \ref{fig:prop_full_overlapping_diff_a}

\begin{lemma}
\label{lem:sum_to_0}
For any number $n>1$ exist set of user vector embedding $U$ of size $n$ which holds:
\begin{align*}
    \sum_{u\in U} u = \overrightarrow{0}
\end{align*}
Where $\overrightarrow{0}$ is the 0 vector.
\proof
We prove the proposition for $d=2$. For $d >2$ we can use the first two dimensions and the other $d-2$ are 0 for all features.
if $n=2$ we define U as follows:
\begin{align*}
    & U = \{u_1, u_2\}\\
    & u_1 = (-1, 0) \\
    & u_2 = (1, 0)
\end{align*}
Note that $\sum_{u\in U} u = u_1 + u_2 = (0, 0)$. \\
if $n=3$ we define U as follows:
\begin{align*}
    & U = \{u_1, u_2, u_3\}\\
    & u_1 = (\frac{1}{2}, \frac{\sqrt{3}}{2}) \\
    & u_2 = (\frac{1}{2}, -\frac{\sqrt{3}}{2}) \\
    & u_3 = (-1, 0)
\end{align*}
Note that $\sum_{u\in U} u = u_1 + u_2 + u_3 = (0, 0)$. \\
Observation:  $\forall n > 1$ $\exists \alpha, \beta \ge 0$ that holds:
\begin{align*}
n = 2\alpha + 3\beta
\end{align*}
Thus, for vector set $U$ of size $n > 1$ we can decompose the vector on it to $\alpha$ subsets of size 2 and $beta$ subsets of size 3. 
The embedding vectors in the subsets of size 2 and 3 are defined as above. The summation of the vector of each subset is $(0, 0)$ and since $U$ is consist by all of those subsets we get:
\begin{align*}
    \sum_{u\in U} u = (0, 0)
\end{align*}
\endproof
\end{lemma}

\subsection{proposition 2}
\label{apx:proof_diff_users_max_div}
First we prove that for $|U|>1$ the diversity is 1.\\
According to the lemma above (\ref{lem:sum_to_0}) exist set of user embedding vectors $U$ of size $|U_1 \bigcap U_2|$ that holds:
\begin{align*}
    \sum_{u\in U} u = \overrightarrow{0}
\end{align*}
We define $f$ that assign to each user in $|U_1 \bigcap U_2|$ vector in $U$ (one to one map).
% We denote in $u_1$ the embedding vector of the user that in $U_1$ but not in $U_2$. In addition we denote in $u_2$ the embedding vector of the user in $U_2$ but not in $U_1$. \\
Since the sum of the vectors in $U$ is 0 it holds:
\begin{align*}
    & \vtilde_1 = u_1 \\
    & \vtilde_2 = u_2
\end{align*}
There is no cost restriction thus the strategic response of items according to \eqref{eq:Delta_closed_form} is as follows: 
\begin{align*}
    & \Delta_f(x_1) = u_1 \\
    & \Delta_f(x_2) = u_2
\end{align*}
In order to create diversity between $\Delta_f(x_1)$ and  $\Delta_f(x_1)$ that is 1 we can use any choice of vectors $u_1$ and $u_2$ that holds: $u_1 = -u_2$.\\
% For the case that $|U|=1$ we i.e $U={u}$ we assign to $u_1$ and $u_2$ the following vectors:
% \begin{align*}
%     & u_1 = -u - \delta \\
%     & u_2 = -u + \delta 
% \end{align*}
% Where $\delta > 0$. 
\endproof

\subsection{proposition 3}
\label{apx:proof_div_multi_list}
We prove the proposition for $d=2$. For $d >2$ we can use the first two dimensions and the other $d-2$ are 0 for all features. We construct the following graph with the following user vector embedding: \\
The user $i$'s list of candidate items contains the items $x_i, x_{i+1}$ for all $i< N$. For user $N$ the items in the list are $x_N, x_1$. \\
Let $0<\delta$. Since our example is in 2 dimensions we can define the user vector embedding with an angle instead of explicitly feature importance vector. Furthermore, we label the features with x and y according to the Cartesian axis. We define the following embedding: \\
For every odd $i < N$:
\begin{align*}
& u_i = 90 - i\delta 
\end{align*}
For every even $i < N$:
\begin{align*}
& u_i = 270 - i\delta 
\end{align*}
For $i=N$ we define $u_N$:
\begin{align*}
    & u_N = 270 + \delta
\end{align*}

Note that this definition set $x_1$ in $(1, 0)$ since the two users that influence it are $u_1$ and $u_N$ and when we average on those two we get:
\begin{align*}
x: \quad & 
\frac{1}{2}(cos(270+\delta)+cos(90-\delta))= \\
& \frac{1}{2}(cos(-90+\delta)+cos(90-\delta))= \\
& \frac{1}{2}(cos(-(90-\delta)+cos(90-\delta))= \\
& \frac{1}{2}(cos((90-\delta)+cos(90-\delta))= \\
& cos(90-\delta)\\ 
    y: \quad & \frac{1}{2}(sin(270+\delta)+sin(90-\delta))= \\
& \frac{1}{2}(sin(-90+\delta)+sin(90-\delta))= \\
& \frac{1}{2}(-sin(90-\delta)+sin(90-\delta))= \\
& = 0
\end{align*}
This item's y value is 0 and since every item is a unit vector $x_1 = (1,0)$ \\ 
We calculate the response of $x_i$ when $i$ is even for all $1<i<N$. The user that item $x_i$ is trying to satisfy are:
\begin{align*}
& u_{i-1} = 90 - (i-1)\delta \\
& u_i = 270 - i\delta 
\end{align*}
We average the two vector by average each coordinate $x,y$.
\begin{align*}
 x: \quad &  \frac{1}{2}(cos(270 - i\delta) + cos(90-(i - 1)\delta))= \\
& cos(\frac{360-(2i-1)\delta}{2})cos(\frac{180-\delta}{2}) =  \\ 
& cos(180 - \frac{2i-1}{2}\delta)cos(90-\frac{\delta}{2})= \\ 
& -cos(\frac{2i-1}{2}\delta)sin(\frac{\delta}{2}) \\
y: \quad & \frac{1}{2}(sin(270-i\delta)+sin(90-(i-1)\delta)= \\
& sin(\frac{360-(2i-1)\delta}{2})cos(\frac{180-\delta}{2})= \\ 
& sin(180-\frac{2i-1}{2}\delta)cos(90-\frac{\delta}{2})= \\
& sin(\frac{2i-1}{2}\delta)sin(\frac{\delta}{2}) 
\end{align*}
We normalize the average vector to unit length:
\begin{align*}
    & \sqrt{(-cos(\frac{2i-1}{2}\delta)sin(\frac{\delta}{2}))^2 + (sin(\frac{2i-1}{2}\delta)sin(\frac{\delta}{2}))^2} = \\
    & sin(\frac{\delta}{2})\sqrt{cos(\frac{2i-1}{2}\delta)^2 + sin(\frac{2i-1}{2}\delta)^2} = \\
    & sin(\frac{\delta}{2})
\end{align*}

Note that this result must be positive since it is a length of vector and since $0<\delta<180$ the length is $sin(\frac{\delta}{2})$ and not $-sin(\frac{\delta}{2})$.
The normalized vector is:
\begin{align*}
    & (-cos(\frac{2i-1}{2}\delta), sin(\frac{2i-1}{2}\delta)) = \\
    & (cos(180-\frac{2i-1}{2}\delta), sin(180-\frac{2i-1}{2}\delta))
\end{align*}
 Since $\alpha=0$ according to \eqref{eq:Delta_closed_form} this is the coordinate of $\Delta(x_i)$. 

We calculate the response of $x_i$ when $i$ is odd for all $1<i<N$. The user that item $x_i$ is trying to satisfy are:
\begin{align*}
& u_{i-1} = 270 - (i-1)\delta \\
& u_i = 90 - i\delta 
\end{align*}

We average the two vector by average each coordinate $x,y$.
\begin{align*}
 x: \quad &  \frac{1}{2}(cos(270 - (i-1)\delta) + cos(90-i\delta)= \\
& cos(\frac{360+(1-2i)\delta}{2})cos(\frac{180+\delta}{2}) =  \\ 
& cos(180 - \frac{2i-1}{2}\delta)cos(90+\frac{\delta}{2})= \\ 
& cos(\frac{2i-1}{2}\delta)sin(\frac{\delta}{2}) \\
y: \quad & \frac{1}{2}(sin(270-(i-1)\delta)+sin(90-i\delta)= \\
& sin(\frac{360-(2i-1)\delta}{2})cos(\frac{180+\delta}{2})= \\ 
& sin(180-\frac{2i-1}{2}\delta)sin(-\frac{\delta}{2})= \\
& -sin(\frac{2i-1}{2}\delta)sin(\frac{\delta}{2}) 
\end{align*}
We normalize the average vector to unit length:
\begin{align*}
    & \sqrt{(cos(\frac{2i-1}{2}\delta)sin(\frac{\delta}{2}))^2 + (-sin(\frac{2i-1}{2}\delta)sin(\frac{\delta}{2}))^2} = \\
    & sin(\frac{\delta}{2})\sqrt{cos(\frac{2i-1}{2}\delta)^2 + sin(\frac{2i-1}{2}\delta)^2} = \\
    & sin(\frac{\delta}{2})
\end{align*}

The normalized vector is:
\begin{align*}
    & (cos(\frac{2i-1}{2}\delta), -sin(\frac{2i-1}{2}\delta)) = \\
    & (cos(-\frac{2i-1}{2}\delta), sin(-\frac{2i-1}{2}\delta))
\end{align*}
Since $\alpha=0$ according to \eqref{eq:Delta_closed_form} this is the coordinate of $\Delta(x_i)$. 

We now calculate the diversity for each user $i < N-1$.\\
User 1 has items $x_1$ and $x_2$ in his recommendation list. Thus diversity should be:
\begin{align*}
    & \frac{1-x_1^Tx_2}{2} = \\
    & \frac{1}{2}(1-(1 \cdot (-cos(\frac{4-1}{2}\delta) + 0 \cdot sin(\frac{4-1}{2}\delta))) = \\
    & \frac{1 + cos(\frac{3\delta}{2})}{2}
\end{align*}
For calculating the diversity in the recommendation list of user i when i is even we first calculate the cosine similarity:
% \begin{align*}
%     & x_i^Tx_{i-1} = \\
%     & cos(180-\frac{2i-1}{2}\delta)cos(-\frac{2(i-1)-1}{2}\delta)+  sin(180-\frac{2i-1}{2}\delta)sin(-\frac{2(i-1)-1}{2}\delta) = \\
%     & cos(180-\frac{2i-1}{2}\delta)cos(-\frac{2i-3}{2}\delta)+  sin(180-\frac{2i-1}{2}\delta)sin(-\frac{2i-3}{2}\delta) = \\
%     & cos(180-\frac{2i-1}{2}\delta)cos(\frac{2i-3}{2}\delta)-sin(\frac{2i-1}{2}\delta)sin(\frac{2i-3}{2}\delta) = \\
%     & -\frac{1}{2}(cos((2i-2)\delta)+cos(\delta)-cos((2i-2)\delta)+cos(\delta)) = \\
%     & -cos(\delta)
% \end{align*}

\begin{align*}
    & x_i^Tx_{i+1} = \\
    & -cos(\frac{2i-1}{2}\delta)cos(-\frac{2(i+1)-1}{2}\delta) + sin(\frac{2i-1}{2}\delta)sin(-\frac{2(i+1)-1}{2}\delta) = \\
    & -cos(\frac{2i-1}{2}\delta)cos(-\frac{2i+1}{2}\delta)+  sin(\frac{2i-1}{2}\delta)sin(-\frac{2i+1}{2}\delta) = \\
    & -[cos(\frac{2i-1}{2}\delta)cos(-\frac{2i+1}{2}\delta)-  sin(\frac{2i-1}{2}\delta)sin(-\frac{2i+1}{2}\delta)] = \\
    & -cos(\frac{2i-1}{2}\delta -\frac{2i+1}{2}\delta) = \\
    & -cos(\delta)
\end{align*}

And the diversity can now be calculated:
\begin{align*}
& \frac{1-x_i^Tx_{i-1}}{2} = \frac{1+cos(\delta)}{2}    
\end{align*}
For calculating the diversity in the recommendation list of user i when i is odd we first calculate the cosine similarity:
% \begin{align*}
%     & x_i^Tx_{i-1} = \\
%     & cos(-\frac{2i-1}{2}\delta)cos(180-\frac{2(i-1)-1}{2}\delta) + sin(-\frac{(2i-1)\delta}{2})sin(180-\frac{(2(i-1)-1)\delta}{2}) = \\
%     & cos(-\frac{2i-1}{2}\delta)cos(180-\frac{2i-3}{2}\delta) - sin(\frac{(2i-1)\delta}{2})sin(180-\frac{2i-3}{2}\delta) = \\
%     & -\frac{1}{2}(cos((2i-2)\delta)+cos(\delta)-cos((2i-2)\delta)+cos(\delta)) = \\
%     & -cos(\delta)
% \end{align*}

\begin{align*}
    & x_i^Tx_{i+1} = \\
    & -cos(-\frac{2i-1}{2}\delta)cos(\frac{2(i+1)-1}{2}\delta) + sin(-\frac{2i-1}{2}\delta)sin(\frac{2(i+1)-1}{2}\delta) = \\
    & -cos(-\frac{2i-1}{2}\delta)cos(\frac{2i+1}{2}\delta)+  sin(-\frac{2i-1}{2}\delta)sin(\frac{2i+1}{2}\delta) = \\
    & -[cos(-\frac{2i-1}{2}\delta)cos(\frac{2i+1}{2}\delta)-  sin(-\frac{2i-1}{2}\delta)sin(\frac{2i+1}{2}\delta)] = \\
    & -cos(-\frac{2i-1}{2}\delta +\frac{2i+1}{2}\delta) = \\
    & -cos(\delta)
\end{align*}

And the diversity can now be calculated:
\begin{align*}
& \frac{1-x_i^Tx_{i-1}}{2} = \frac{1+cos(\delta)}{2}    
\end{align*}
The last two users to calculate the diversity are the $N-1$'th user and $N$'th user.
% Which depends if $N$ is odd or even (in order to know the vector $u_m$). We will mark the diversity of the recommendation list for user $m$ in $d_m$.\\
We mark the diversity of those two users in $d_{N-1}$ and $d_N$.
The overall diversity according to \eqref{eq:divk} is:
\begin{align*}
    \DIV = \frac{1}{N}(d _{N-1} + d_N +\frac{1 + cos(\frac{3\delta}{2})}{2} + \frac{(N-3)(1+cos(\delta))}{2}) 
\end{align*}
Since $d_{N-1}$ and $d_N$ are not negative thus we get:
% and $\frac{1 + cos(\frac{3\delta}{2})}{2}$ is not negative thus we get:
\begin{align*}
\DIV \ge \frac{1}{N} (\frac{1 + cos(\frac{3\delta}{2})}{2} + \frac{(N-3)(1+cos(\delta))}{2})
\end{align*}
$\frac{1 + cos(\frac{3\delta}{2})}{2}$ is also not negative since $cos(\frac{3\delta}{2})$ is not less than -1. We get:
\begin{align*}
\DIV \ge \frac{(N-3)(1+cos(\delta))}{2N} = \frac{N-3}{N}\frac{1+cos(\delta)}{2}
\end{align*}
We choose $\delta = cos^{-1}(1-2\epsilon)$ which means $\epsilon = \frac{1-cos(\delta)}{2}$ and since $1-\epsilon = \frac{1+cos(\delta)}{2}$ we get:
\begin{align*}
\DIV \ge \frac{N-3}{N}(1-\epsilon)
\end{align*}
\endproof

\section{Additional experimental results: synthetic data}
\label{apx:additional_result}

\subsection{Time vs. modification costs: diversification in depth}
For our experiment in Sec. \ref{sec:synth_vary_costs},
Fig. \ref{apx:fig:angles} visualizes for a set of items in $\R^2$ how they quickly become dispersed.

\begin{figure}[h!]
    \centering
    \includegraphics[width=0.4\textwidth]{synthetic_exp_plots/angle dispersion 3.pdf}
    \caption{
    Dispersal of items $x_i \in \R^2$ over time.
    }
    \label{apx:fig:angles}
\end{figure}

\subsection{Performance over time}
\label{multi_rounds}
This experiment examines how diversity changes over several rounds. The results of this experiment are shown in figure \ref{fig:synth_round}. For $\lambda=0$ (no diversity is added to learning), the model's NDCG is high and fixed. Since we use a small  $\sigma_{u^*}$, the strategic responses of the items are almost the same, which leads to a small diversity (as in experiment \ref{variation_u*}) .
 As a contrast, when $\lambda = 1000$ and diversity is primarily considered, we can observe that diversity increases to a high value at the first round  
 % \red{(round 0 in the figure)} 
 and NDCG decreases. In the subsequent rounds, diversity remains high and NDCG remains low. As $\lambda$ decreases, we observe the model tries to balance NDCG and diversity and doesn't sacrifice all NDCG. As $\lambda$ increases, more NDCG is sacrificed and diversity increases. Nevertheless, lower values of $\lambda$ exhibit periodic trends in diversity.\\
To explain why the periodic trend is formed when $\lambda$ is small, we emphasize two special properties of the NDCG-diversity relation:  
\begin{enumerate}[noitemsep,leftmargin=1cm,label=(\arabic*)]
% \item For small values of $\lambda$ when diversity is high items are different from each other. That might cause a significant different in their relevance. As a result small permutation in item list causes NDCG to drop. In order to avoid small NDCG the model has to learn user embedding that are close to $u^*$ which in our case leads to small diversity in the next round.
\item The relevance of items may differ significantly when diversity is high.  As a result, NDCG drops when there is a small permutation in the item list. To avoid small NDCG, the model learns user embeddings close to $u^*$, which leads to small diversity next round.
\item When diversity is low and feature space is small, items' features are very similar, so they have almost the same relevance.
As a result, changes in item order might not significantly harm NDCG.
Consequently, the model may change user embeddings (which affect item order) in an effort to encourage diversity without sacrificing NDCG.
\end{enumerate}
We can explain the periodic trends for small values of $\lambda$ using those two properties. The model prefers NDCG over diversity when $\lambda=0.025$. As with $\lambda = 0$, the strategic response in the first round leads to a small diversity in the second round. Diversity in the third round is high according to property 2, while diversity in the fourth round is low according to property 1. A periodic trend can be observed: 
Odd rounds diversity is low while in even rounds diversity is high.

\begin{figure*}[t!]
\label{fig:synth_round}
\centering
\includegraphics[width=0.4\textwidth]{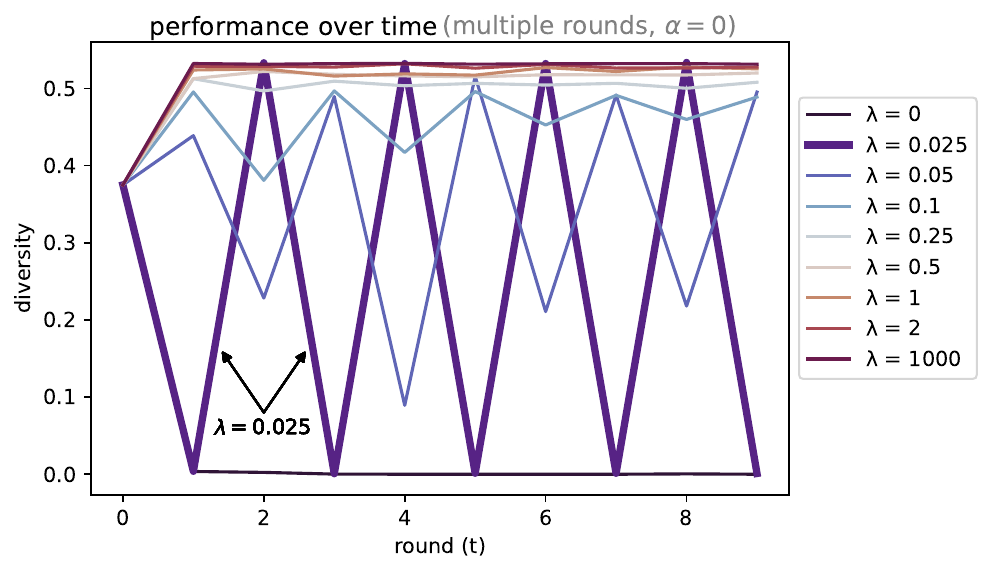} \qquad
\includegraphics[width=0.4\textwidth]{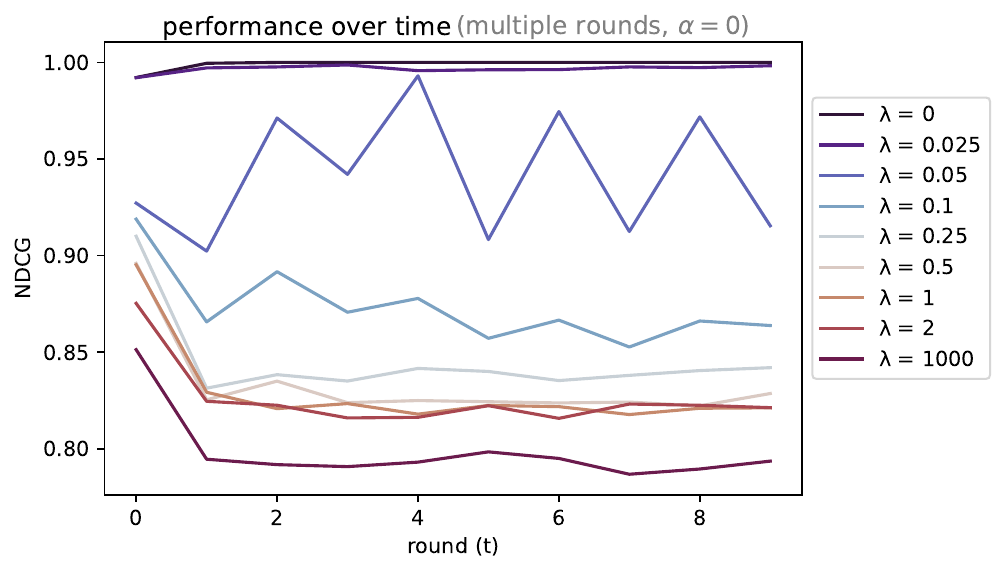}
\caption{\textbf{(Left)} diversity vs number of rounds. \textbf{(Right)} NDCG vs number of rounds.}
\label{fig:synth time}
\end{figure*}

\subsection{The affect of $k$ in topk diversity}
We aim to understand how the size of the recommendation list $k$ impacts the ability of the model to create diversity. We repeated the previous experiment, but changed the parameter $k$. Fig. \ref{fig:synth k time} compares two values of $\lambda$, the first being low ($\lambda=0.025$, which is not 0) and the second being high ($\lambda=1$). We see that low values of $k$ result in lower diversity, which means it is harder for the model to obtain high diversity. The reason for this might be that our model ranks items based on linear equations for each user, which may cause similar items to appear first. When $k$ is small, there are few items at the top of the list that may be similar to others.
% \red{do we really want to admit it?? that explains why diversity decrease after strategic movement} 
In the previous experiment \ref{multi_rounds}, we saw that for $k=10$ and high $\lambda$, model diversity was high and steady, whereas for low $\lambda$, there was periodic trending.
%The figures show that in cases that $k < 10$,
% retraining of the model (before strategic movement) leads to a decrease in diversity when $k$ is less than 10.
The figures demonstrate that when $k < 10$, retraining the model at the end of each round causes a change in diversity since the items are reordered in a different way to increase current NDCG and ensure high diversity in the next round.
As a result of the reordering, the set of items included in the top k of the list has changed, which may affect diversity.
% Due to reordering, some of the items that were included in the top k of the list are not included any more which might cause some change in the diversity. 

% After the model is re-trained at the end of each round, some items that were very different from each other might rank lower than $k$ since the items are reordered before the strategic movement. Those items that were previously taken into account are no longer included in the topk diversity calculation.
% For $k=2$, re-training does not seem to change the diversity much; however, this might be because $k$ is low, which means that two items at the top might be similar, so the re-order does not make much difference. 

\begin{figure*}[t!]
\centering
\includegraphics[width=0.4\textwidth]{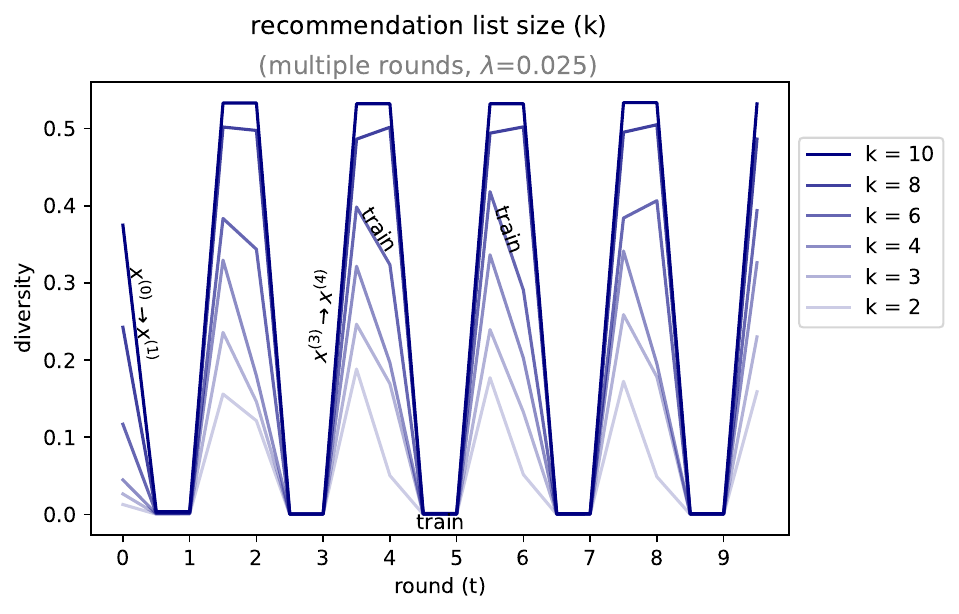} \qquad
\includegraphics[width=0.4\textwidth]{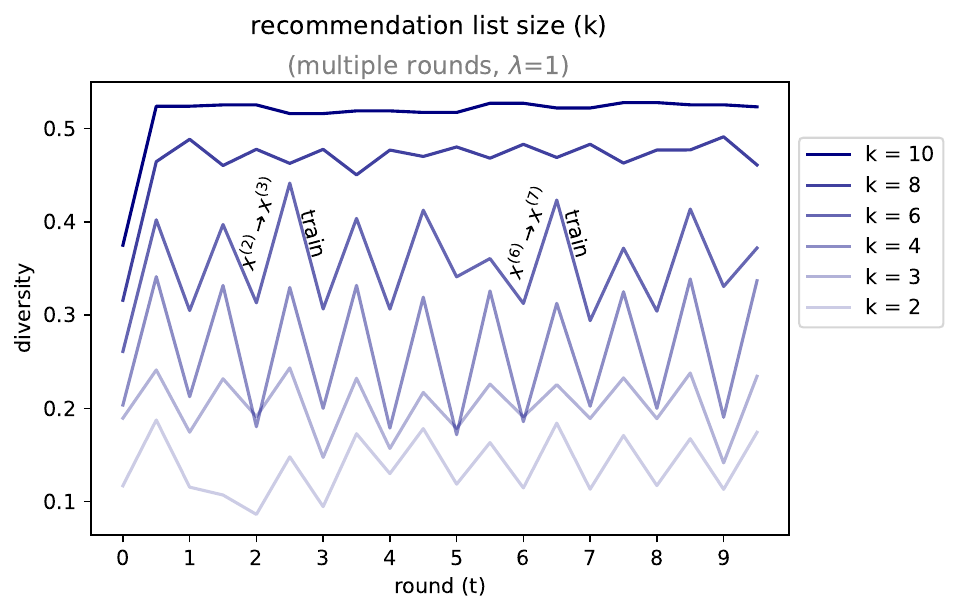}
\caption{\textbf{(Left)} diversity vs number of rounds for $\lambda=0.025$. \textbf{(Right)} diversity vs number of rounds for $\lambda=1$.}
\label{fig:synth k time}
\end{figure*}

\section{Experimental details}
\label{apx:Data details}
\subsection{Yelp dataset and restaurant features} 
\paragraph{Restaurants.} This dataset contains information about businesses. There is a list of categories that might be relevant to each business. In our experiment, we used only restaurants. In order to find all the restaurants, we manually search all possible categories that might be assigned to restaurant categories, such as Pizza or Burgers. Business is removed if it hasn't been in one of those categories. We left with 22,197 restaurants. We grouped similar categories with the same meaning, such as Pita, Turkish, Falafel, Ersian/Iranian, Syrian, Egyptian, Arabian, Lebanese and Kebab into "middle east". It is considered that restaurants with this category have value 1 in the feature "middle east". \\

\paragraph{User and reviews information}
A total of 740434 users have written reviews. Our experiments required users to review many restaurants (A recommendation list is based on past interactions between a user and a restaurant). In our experiment, only users who have reviewed at least 100 different restaurants were included. After that filter, 236 users are left.

% number of users in 740434

\subsection{Recommendation list creation}
\label{apx: recommendation list creation}
As we mentioned above, only users who wrote reviews for 100 different restaurants were included in our experiment (236 users). Due to this filter, there are many restaurants that left with only one user ranking them. Therefore, the strategic responses of those restaurants were influenced only by this user's embedding.
This is an unrealistic distortion that could have harm the correctness of our results. 
We wanted to reduce those cases and at the same time reduce the size of the recommendation list to be 40 (that reduce the running time of our experiment). Thus we used the following algorithm to create users recommendation list: \\
Let $R$ be set of restaurants and $U$ be the set of users who reviewed 100 different restaurants. 
\begin{enumerate}
    \item For all user $u$ set the recommendation list to $\emptyset$
    \item For each restaurant $r$, create a set of users $r_u$ that have reviewed the restaurant reviewed this. 
    % \item Given a sentence of length $l$, for $i = 0, 1, ...., l$:
    \item Until exist user with less than 40 restaurant in the recommendation list:
    \begin{enumerate}
        \item Pick the restaurant $r$ with the most users in $U$.
        \item For each user $u \in r_u$: 
        \begin{enumerate}
            \item Add the restaurant to the recommendation list of user $u$.
            \item $R = R  - \{r\}$
            \item If the recommendation list contains 40 items:
            \begin{enumerate}
                \item for each restaurant $r'$ that $u$ reviewed:
                \item Remove $u$ from $r'_u$.
            \end{enumerate}
        \end{enumerate}
    \end{enumerate}
\end{enumerate}
% To overcome this problem we sorted all the restaurants according to the number of users the reviewed them. 
\subsection{Training the ground truth model $f^*$}
\label{apx:training f^*}
\paragraph{purpose.} The function $f^*$ assigns a score to item $x$ in relation to a user with features $u^*$. The higher the score, the more relevant the item is to the user. As the information we have about the restaurant focuses mainly on technical details, and the enjoyment of users depends on a range of random factors, we do not expect to be able to predict user rankings. Instead, we search for restaurants the user might be interested in visiting. $f^*$ calculate to each pair $u^*, x$ score in $\R$. When the score is greater than 0.5, we consider the user might be interested in visiting the restaurant and when the score is less than 0.5, we consider the user probably won't be interested in visiting this restaurant. \paragraph{User features.} There were no features to be included in our data for users. Using information on user previous interactions, we provided features to users. Every restaurant feature was averaged across all restaurants visited by a user. It means that the vector feature of user $i$ $u_i^*$ is calculated as follows:
\begin{align*}
    u_i^* = \frac{\sum_{x\in \rev{(u_i)}}x}{{|\rev{(u_i)}|}}
\end{align*}
$\rev(u_i)$ represents all restaurants that the user has reviewed.
\paragraph{Train and evaluation $f^*$.} In order to train $f^*$ we used all the reviews of user that reviewed at least 50 restaurants. After that filter we had 1377 users and 113852 reviews. Since each review (whenever is positive or negative) indicates that user visit the restaurant (i.e the user interested the restaurant) thus we tagged it as a positive example. In order to get negative examples we used the coordinate of each restaurant (that is included in the dataset) and search for each review the closest restaurant that the user didn't review. Since the restaurant are close could choose to visit the one without the review but choose not to. We split the reviews to train set, validation set and test set. The train set includes 70\% of the reviews, the validation set includes 20\% of the reviews and the test set includes 10\%. As part of our training process, we used Adam optimizer with learning rate 0.01 to enable the model to converge to useful weights in a reasonable amount of time. The number of epoch to train was set using the validation set. The final evaluation was made on the test set and it received 72\% accuracy.
\paragraph{Model structure.} We used MLP architecture to $f^*$. Each layer consist a linear transformation and a Relu function. There were five layers in the model, which seems to be sufficient to capture non-linear interaction between user vector features and items.
%We empirically choose 5 linear layers.% 
The first layer gets 86 features as input (43 as restaurant features and 43 as user feature) and the output dimension is 172 (twice bigger than the input). The rest of the layers reduce the number of features by half (each layer reduce by half).

% \subsection{Training recommendation system}
% In \ref{apx: recommendation list creation} we described how we created for each user items list. However while we trained the model to each user we used subset of those items which randomly chosen. The evaluation was made in the entire list of items which measured the ability of the model to deal with unseen items. We used Adam optimizer \red{Add a citation after Nir enters his changes} in the training phase. We trained the model 200 epochs  

\subsection{Training recommendation system}
% Our experiments include dynamic process over the time where each even time stamp the RS trains and each odd time stamp the items has been change according the trained RS model. As we described in section \ref{sec:real data} we preform our experiment over 20 time stamps which means that we trained 20 different models.\\ 
\textbf{Training hyper parameters.} As we described in section \ref{sec:real data} we preform our experiment over 20 time stamps which means that we trained 20 different models. The model were trained over 200 epochs using Adam optimizer. Our learning rate is set at 0.1, which allows the model to achieve good results in a reasonable amount of time. In order to optimize equation \eqref{eq:learning_objective_strat} We had to use two smooth permutation matrices one to optimize NDCG and the other for diversity. In order to get accurate NDCG we used relatively small $\tau=0.1$. In order to optimize diversity, it is necessary to consider all items' strategic responses, which may complicate the optimization process. Thus, we optimize diversity using a large tau values ($\tau=1$ for the approx permutation matrix and 5 for the $\sigma_\tau$ function), as it is easier to optimize.\\
\textbf{Computational infrastructure.} All experiments were run on cluster ( AMD EPYC 7713 64, 1568 Mhz, 256 core \red{RAM}). %ram
 
\section{Additional experimental results: real data}
\label{apx:results_real}

\subsection{Dynamics}
\begin{figure*}[t!]
\centering
\includegraphics[width=\textwidth]{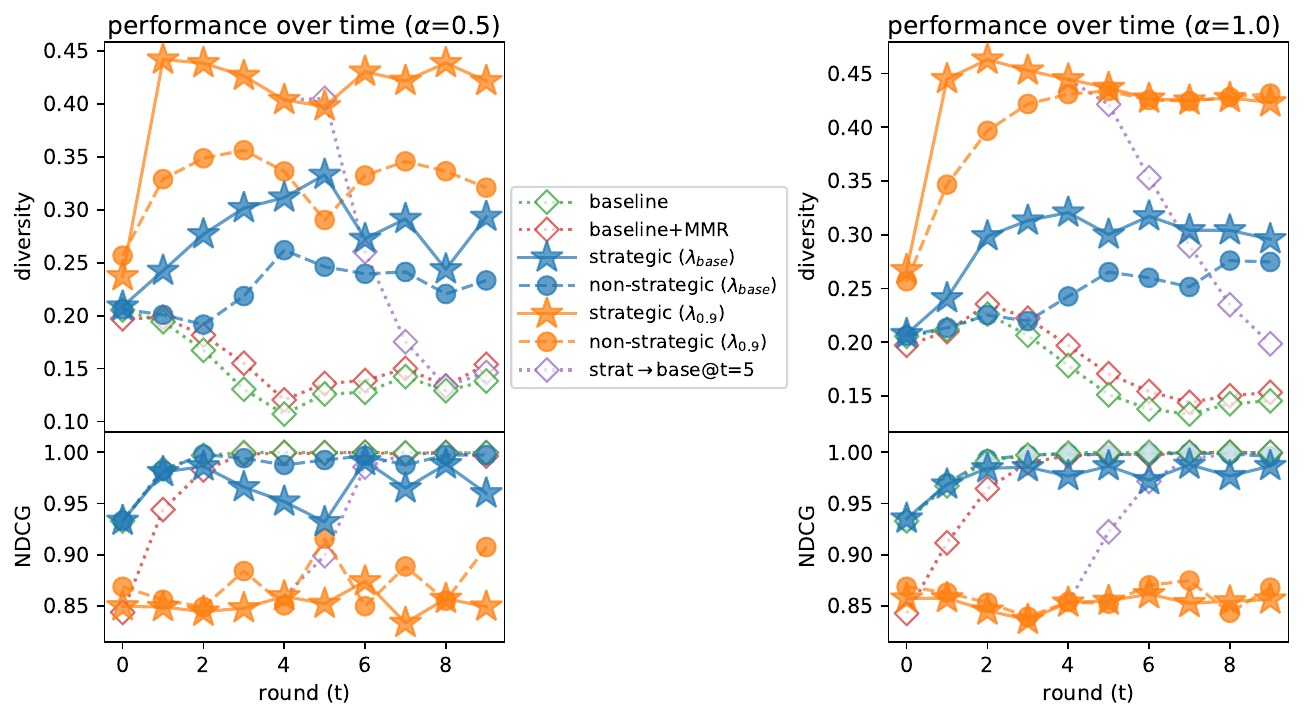}
\caption{\textbf{(Left)} diversity vs number of rounds. \textbf{(Right)} NDCG vs number of rounds.}
\end{figure*}

\subsection{NDCG diversity tradeoff}
\red{here I should insert result of low $\alpha$ but when $\alpha$ is small the trde off after the strategic change a little strange. If I put $\alpha =0.5$ it looks good but for lower sometimes higher NDCG get higher diversity..}
